# Supplementary material for: Anatomy of spin-orbit-torque-assisted magnetization dynamics in Co/Pt bilayers: Importance of the orbital torque
Source: arXiv:2505.17698 source file (2025-10-04)
Supplement: Supplementary file 1 [file SOT_Pt_Co_supplemental.pdf]

# Supplemental Material for
# Anatomy of spin-orbit-torque-assisted magnetization dynamics in Co/Pt bilayers: Importance of the orbital torque

Harshita Devda*[,1], András Deák[2], Leandro Salemi[3], Levente Rózsa[4,2], László Szunyogh[2,5], Peter M. Oppeneer[3], and Ulrich Nowak[1]
*harshita.devda@uni-konstanz.de
[1]Fachbereich Physik, Universität Konstanz, DE-78457 Konstanz, Germany
[2]Department of Theoretical Physics, Institute of Physics, Budapest University of Technology and Economics, Muegyetem rkp. 3, 1111 Budapest, Hungary
[3]Department of Physics and Astronomy, Uppsala University, P. O. Box 516, S-751 20 Uppsala, Sweden
[4]Department of Theoretical Solid State Physics, HUN-REN Wigner Research Centre for Physics, 1525 Budapest, Hungary and
[5]HUN-REN-BME Condensed Matter Research Group, Budapest University of Technology and Economics, Muegyetem rkp. 3, 1111 Budapest, Hungary

## I. RENORMALIZATION OF THE SPIN-MODEL PARAMETERS

In the spirit of Refs. [1] and [2], here we give a detailed derivation of the renormalized spin Hamiltonian, Eqs. (4)-(6) in the main text. In the classical spin model of the Pt/Co bilayer, the strong Co spin magnetic moments of magnitudes $\mu^d_{S,i}$ are represented by unit vectors $\boldsymbol{S}_i$ with $\boldsymbol{\mu}^d_{S,i} = \mu^d_{S,i}\boldsymbol{S}_i$. In order to include longitudinal spin fluctuations of the induced Pt spin moments, those are treated as three-dimensional vectors $\boldsymbol{\mu}_{S,\nu}$. In our model we consider on-site anisotropy at the Co sites, tensorial exchange interactions between the Co spins as well as between Co and Pt moments, and the formation energy of the induced Pt moments,

$$\mathcal{H}(\{\boldsymbol{S}_i\},\{\boldsymbol{\mu}_{S,\nu}\}) = \sum_i \boldsymbol{S}_i\mathcal{K}_i\boldsymbol{S}_i - \frac{1}{2}\sum_{i\neq j}\boldsymbol{S}_i\mathcal{J}_{ij}\boldsymbol{S}_j - \sum_{i\nu}\boldsymbol{S}_i\mathcal{L}_{i\nu}\boldsymbol{\mu}_{S,\nu} + \sum_\nu \mathcal{H}_\nu(\boldsymbol{\mu}_{S,\nu})\,, \tag{S1}$$

where $\mathcal{K}_i$, $\mathcal{J}_{ij}$ and $\mathcal{L}_{i\nu}$ are $3\times 3$ matrices with the properties $\mathcal{K}_i = \mathcal{K}_i^T$, $\mathcal{J}_{ji} = \mathcal{J}_{ij}^T$ and $\mathcal{L}_{\nu i} = \mathcal{L}_{i\nu}^T$. Note that the exchange coupling tensors $\mathcal{J}_{ij}$ and $\mathcal{L}_{i\nu}$ have different dimensions. For the formation energy of the Pt spin moments we use the simplest approximation,

$$\mathcal{H}_\nu(\boldsymbol{\mu}_{S,\nu}) = a_\nu \boldsymbol{\mu}^2_{S,\nu}\,, \tag{S2}$$

where the coefficients $a_\nu > 0$ will be fixed later on.

When a static electric field $\boldsymbol{E}$ is applied, additional spin magnetic moments,

$$\delta\boldsymbol{\mu}_{S,i} = \boldsymbol{\chi}^S_i\cdot\boldsymbol{E} \quad\text{and}\quad \delta\boldsymbol{\mu}_{S,\nu} = \boldsymbol{\chi}^S_\nu\cdot\boldsymbol{E}\,, \tag{S3}$$

and orbital magnetic moments,

$$\delta\boldsymbol{\mu}_{L,i} = \boldsymbol{\chi}^L_i\cdot\boldsymbol{E} \quad\text{and}\quad \delta\boldsymbol{\mu}_{L,\nu} = \boldsymbol{\chi}^L_\nu\cdot\boldsymbol{E}\,, \tag{S4}$$

are induced on the Co and Pt sites, respectively. We suppose that the electrically induced spin moments form an additive contribution to the original strong spin moments at the Co atoms, thus, the total spin moment at site $i$ is $\boldsymbol{\mu}^d_{S,i} + \delta\boldsymbol{\mu}_{S,i}$. The exchange interaction between the strong Co spin moments at sites $i$ and $j$ can be written as

$$\boldsymbol{S}_i\mathcal{J}_{ij}\boldsymbol{S}_j = \boldsymbol{\mu}^d_{S,i}\frac{\mathcal{J}_{ij}}{\mu^d_{S,i}\mu^d_{S,j}}\boldsymbol{\mu}^d_{S,j}\,, \tag{S5}$$

and we assume that the coupling strengths $\mathcal{J}_{ij}/\mu^d_{S,i}\mu^d_{S,j}$ are independent of the magnitudes of the spin moments. The exchange interaction can then be extended to the case of nonzero electric field as

$$\begin{aligned}(\boldsymbol{\mu}^d_{S,i} + \delta\boldsymbol{\mu}_{S,i})\frac{\mathcal{J}_{ij}}{\mu^d_{S,i}\mu^d_{S,j}}(\boldsymbol{\mu}^d_{S,j} + \delta\boldsymbol{\mu}_{S,j}) &\simeq \boldsymbol{S}_i\mathcal{J}_{ij}\boldsymbol{S}_j + \frac{1}{\mu^d_{S,i}}\delta\boldsymbol{\mu}_{S,i}\mathcal{J}_{ij}\boldsymbol{S}_j + \frac{1}{\mu^d_{S,j}}\boldsymbol{S}_i\mathcal{J}_{ij}\delta\boldsymbol{\mu}_{S,j}\\ &= \boldsymbol{S}_i\mathcal{J}_{ij}\boldsymbol{S}_j + \frac{1}{\mu^d_{S,i}}\delta\boldsymbol{\mu}_{S,i}\mathcal{J}_{ij}\boldsymbol{S}_j + \frac{1}{\mu^d_{S,j}}\delta\boldsymbol{\mu}_{S,j}\mathcal{J}_{ji}\boldsymbol{S}_i\,,\end{aligned} \tag{S6}$$

where we neglected the term proportional to the square of the electric field which is independent of the spin configuration. The sum of the exchange interaction energies can be expressed as

$$-\frac{1}{2}\sum_{i\neq j}(\boldsymbol{\mu}^d_{S,i}+\delta\boldsymbol{\mu}_{S,i})\frac{\mathcal{J}_{ij}}{\mu^d_{S,i}\mu^d_{S,j}}(\boldsymbol{\mu}^d_{S,j}+\delta\boldsymbol{\mu}_{S,j}) \simeq -\frac{1}{2}\sum_{i\neq j}\boldsymbol{S}_i\mathcal{J}_{ij}\boldsymbol{S}_j - \sum_i\sum_{j(\neq i)}\frac{1}{\mu^d_{S,j}}\delta\boldsymbol{\mu}_{S,j}\mathcal{J}_{ji}\boldsymbol{S}_i$$
$$= -\frac{1}{2}\sum_{i\neq j}\boldsymbol{S}_i\mathcal{J}_{ij}\boldsymbol{S}_j - \sum_i \mu^d_{S,i}\boldsymbol{b}^E_{S,i}\boldsymbol{S}_i\,, \tag{S7}$$

with the electrically induced effective fields at the Co sites,

$$\boldsymbol{b}^E_{S,i} = \sum_{j(\neq i)}\frac{\mathcal{J}_{ij}}{\mu^d_{S,i}\mu^d_{S,j}}\delta\boldsymbol{\mu}_{S,j} = \sum_{j(\neq i)}\frac{\mathcal{J}_{ij}}{\mu^d_{S,i}\mu^d_{S,j}}(\boldsymbol{\chi}^S_j\cdot\boldsymbol{E})\,. \tag{S8}$$

The exchange interaction between the strong Co moments and the induced Pt moments can similarly be expressed in the presence of the electric field,

$$-\sum_{i\nu}\frac{1}{\mu^d_{S,i}}(\boldsymbol{\mu}^d_{S,i}+\boldsymbol{\delta\mu}_{S,i})\mathcal{L}_{i\nu}\boldsymbol{\mu}_{S,\nu} = -\sum_{i\nu}(\boldsymbol{S}_i+\frac{1}{\mu^d_{S,i}}\boldsymbol{\chi}^S_i\boldsymbol{E})\mathcal{L}_{i\nu}\boldsymbol{\mu}_{S,\nu}\,, \tag{S9}$$

where $\boldsymbol{\mu}_{S,\nu}$ stands for the total induced Pt spin magnetic moment due to both the exchange with the Co spins and the spin-polarization effect of the electric field. The latter one contains a contribution from the exchange interaction with the electrically induced Co moments included in the previous term. The contribution related to a direct spin-polarization effect at the Pt sites is taken into account through an effective field, $\boldsymbol{b}^{(d)E}_\nu$. Taking into account all the above terms, we extend the Hamiltonian (S1) as

$$\mathcal{H}_S(\{\boldsymbol{S}_i\},\{\boldsymbol{\mu}_{S,\nu}\},\boldsymbol{E}) = \sum_i\boldsymbol{S}_i\mathcal{K}_i\boldsymbol{S}_i - \sum_i\frac{J^{sd}}{\mu^d_{S,i}}\delta\boldsymbol{\mu}_{S,i}\boldsymbol{S}_i - \frac{1}{2}\sum_{i\neq j}\boldsymbol{S}_i\mathcal{J}_{ij}\boldsymbol{S}_j - \sum_i\mu^d_{S,i}\boldsymbol{b}^E_{S,i}\boldsymbol{S}_i$$
$$-\sum_{i\nu}(\boldsymbol{S}_i+\frac{1}{\mu^d_{S,i}}\delta\boldsymbol{\mu}_{S,i})\mathcal{L}_{i\nu}\boldsymbol{\mu}_{S,\nu} - \sum_\nu\boldsymbol{b}^{(d)E}_\nu\boldsymbol{\mu}_{S,\nu} + \sum_\nu\mathcal{H}_\nu(\boldsymbol{\mu}_{S,\nu})\,, \tag{S10}$$

where we also introduced an intra-atomic exchange interaction $J^{sd}$ between the strong moment and the electrically induced spin moment at the Co sites related to electrons occupying $d$ orbitals and $s$ orbitals, respectively. In addition, we add the spin-orbit interaction between the spin magnetic moments and the electrically induced orbital magnetic moments on both the Co and Pt sites,

$$\mathcal{H}_{\mathrm{SOC}}(\{\boldsymbol{S}_i\},\{\boldsymbol{\mu}_{S,\nu}\},\boldsymbol{E}) = \sum_i\frac{\zeta_i}{2\mu_{\mathrm{B}}^2}\boldsymbol{\mu}_{S,i}\cdot\delta\boldsymbol{\mu}_{L,i} + \sum_\nu\frac{\zeta_\nu}{2\mu_{\mathrm{B}}^2}\boldsymbol{\mu}_{S,\nu}\cdot\delta\boldsymbol{\mu}_{L,\nu}$$
$$\simeq \sum_i\frac{\zeta_i}{2\mu_{\mathrm{B}}^2}\mu^d_{S,i}\boldsymbol{S}_i\cdot\delta\boldsymbol{\mu}_{L,i} + \sum_\nu\frac{\zeta_\nu}{2\mu_{\mathrm{B}}^2}\boldsymbol{\mu}_{S,\nu}\cdot\delta\boldsymbol{\mu}_{L,\nu}\,, \tag{S11}$$

where $\zeta_i$ and $\zeta_\nu$ are the spin-orbit coupling strength at the Co and the Pt sites, respectively, and $\mu_{\mathrm{B}}$ is the Bohr magneton. Note that we neglected the spin-orbit interaction between the electrically induced spin and orbital moments of the Co atoms being proportional to the square of the electric field, and the factor of $1/2$ arises from the semi-classical treatment. The total spin Hamiltonian of the Co and Pt spin and orbital moments in the presence of an electric field is then given by

$$\mathcal{H}(\{\boldsymbol{S}_i\},\{\boldsymbol{\mu}_{S,\nu}\},\boldsymbol{E}) = \mathcal{H}_S(\{\boldsymbol{S}_i\},\{\boldsymbol{\mu}_{S,\nu}\},\boldsymbol{E}) + \mathcal{H}_{\mathrm{SOC}}(\{\boldsymbol{S}_i\},\{\boldsymbol{\mu}_{S,\nu}\},\boldsymbol{E})\,. \tag{S12}$$

Supposing that the formation of the induced Pt moments occurs on a much shorter time scale as compared to the slow motion of strong moments, for any configuration of the Co moments $\{\boldsymbol{S}_i\}$ we impose the minimization condition for the Hamiltonian (S1),

$$\left.\frac{\partial\mathcal{H}(\{\boldsymbol{S}_i\},\{\boldsymbol{\mu}_{S,\nu}\},\boldsymbol{E})}{\partial\boldsymbol{\mu}_{S,\nu}}\right|_{\boldsymbol{\mu}^0_{S,\nu}} = 0\,, \tag{S13}$$

we deduce

$$\sum_i\mathcal{L}_{\nu i}(\boldsymbol{S}_i+\frac{1}{\mu^d_{S,i}}\delta\boldsymbol{\mu}_{S,i}) + \boldsymbol{b}^{(d)E}_\nu - 2a_\nu\boldsymbol{\mu}_{S,\nu} - \frac{\zeta_\nu}{2\mu_{\mathrm{B}}^2}\delta\boldsymbol{\mu}_{L,\nu} = 0\,, \tag{S14}$$

from which the total induced spin moments of the Pt atoms can be expressed,

$$\boldsymbol{\mu}^0_{S,\nu} = \frac{1}{2a_\nu}\sum_i \mathcal{L}_{\nu i}\boldsymbol{S}_i + \frac{1}{2a_\nu}\sum_i \frac{1}{\mu^d_{S,i}}\mathcal{L}_{\nu i}\,\delta\boldsymbol{\mu}_{S,i} + \frac{\boldsymbol{b}^{(d)E}_\nu}{2a_\nu} - \frac{1}{2a_\nu}\frac{\zeta_\nu \delta\boldsymbol{\mu}_{L,\nu}}{2\mu_{\mathrm{B}}^2}\,. \tag{S15}$$

The second and third terms are supposed to contribute to the electrically induced spin-moment at the Pt site expressed in terms of the spin susceptibility calculated via linear-response theory,

$$\delta\boldsymbol{\mu}_{S,\nu} = \boldsymbol{\chi}^S_\nu \cdot \boldsymbol{E} = \frac{1}{2a_\nu}\sum_i \frac{1}{\mu^d_{S,i}}\mathcal{L}_{\nu i}\,\delta\boldsymbol{\mu}_{S,i} + \frac{\boldsymbol{b}^{(d)E}_\nu}{2a_\nu}\,. \tag{S16}$$

The last term in Eq. (S15) contains orbital contributions through $\delta\boldsymbol{\mu}^E_{L,\nu} = \boldsymbol{\chi}^L_\nu \cdot \boldsymbol{E}$, thus, it represents a new source for generating spin moments at the Pt sites. We conclude that

$$\boldsymbol{\mu}^0_{S,\nu} = \frac{1}{2a_\nu}(\boldsymbol{b}_{S,\nu} + \boldsymbol{b}^E_{S,\nu} + \boldsymbol{b}^E_{L,\nu})\,, \tag{S17}$$

with the effective fields,

$$\boldsymbol{b}_{S,\nu} = \sum_i \mathcal{L}_{\nu i}\boldsymbol{S}_i\,, \tag{S18}$$

$$\boldsymbol{b}^E_{S,\nu} = 2a_\nu \delta\boldsymbol{\mu}_{S,\nu}\,, \tag{S19}$$

and

$$\boldsymbol{b}^E_{L,\nu} = -\frac{\zeta_\nu}{2\mu_{\mathrm{B}}^2}\delta\boldsymbol{\mu}_{L,\nu}\,. \tag{S20}$$

The terms containing the equilibrium Pt spin moment $\boldsymbol{\mu}^0_{S,\nu}$ in Eq. (S12) can then be combined as follows,

$$\begin{aligned} &-\sum_{i\nu}(\boldsymbol{S}_i + \frac{1}{\mu^d_{S,i}}\delta\boldsymbol{\mu}_{S,i})\mathcal{L}_{i\nu}\boldsymbol{\mu}^0_{S,\nu} - \sum_\nu \boldsymbol{b}^E_{S,\nu}\boldsymbol{\mu}^0_{S,\nu} + \sum_\nu \frac{\zeta_\nu}{2\mu_{\mathrm{B}}^2}\boldsymbol{\mu}^0_{S,\nu}\cdot\delta\boldsymbol{\mu}_{L,\nu} + \sum_\nu \mathcal{H}_\nu(\boldsymbol{\mu}^0_{S,\nu}) \\ &= -\sum_\nu(\boldsymbol{b}_{S,\nu} + \boldsymbol{b}^E_{S,\nu} + \boldsymbol{b}^E_{L,\nu})\boldsymbol{\mu}^0_{S,\nu} + \sum_\nu a_\nu(\boldsymbol{\mu}^0_{S,\nu})^2 = -\sum_\nu \frac{1}{4a_\nu}(\boldsymbol{b}_{S,\nu} + \boldsymbol{b}^E_{S,\nu} + \boldsymbol{b}^E_{L,\nu})^2\,. \end{aligned} \tag{S21}$$

Keeping only the terms which contain $\boldsymbol{b}_{S,\nu}$, i.e., the strong moments $\boldsymbol{S}_i$ explicitly, we can proceed as

$$-\sum_\nu \frac{1}{4a_\nu}(\boldsymbol{b}_{S,\nu} + \boldsymbol{b}^E_{S,\nu} + \boldsymbol{b}^E_{L,\nu})^2 \simeq -\sum_\nu \frac{\boldsymbol{b}^2_{S,\nu}}{4a_\nu} - \sum_\nu \frac{\boldsymbol{b}_{S,\nu}\cdot\boldsymbol{b}^E_{S,\nu}}{2a_\nu} - \sum_\nu \frac{\boldsymbol{b}_{S,\nu}\cdot\boldsymbol{b}^E_{L,\nu}}{2a_\nu}\,. \tag{S22}$$

Adding the term

$$\begin{aligned} -\sum_\nu \frac{\boldsymbol{b}^2_{S,\nu}}{4a_\nu} &= -\sum_\nu \frac{1}{4a_\nu}\sum_{ij}\boldsymbol{S}_i\mathcal{L}_{i\nu}\mathcal{L}_{\nu j}\boldsymbol{S}_j \\ &= -\sum_i \boldsymbol{S}_i(\sum_\nu \frac{1}{4a_\nu}\mathcal{L}_{i\nu}\mathcal{L}_{\nu i})\boldsymbol{S}_i - \frac{1}{2}\sum_{i\neq j}\boldsymbol{S}_i(\sum_\nu \frac{1}{2a_\nu}\mathcal{L}_{i\nu}\mathcal{L}_{\nu j})\boldsymbol{S}_j\,, \end{aligned} \tag{S23}$$

to the first two terms on the right-hand side of Eq. (S10) leads to the renormalization of the on-site anisotropy matrices,

$$\tilde{\mathcal{K}}_i = \mathcal{K}_i - \sum_\nu \frac{1}{4a_\nu}\mathcal{L}_{i\nu}\mathcal{L}_{\nu i}\,, \tag{S24}$$

and the exchange interaction matrices,

$$\tilde{\mathcal{J}}_{ij} = \mathcal{J}_{ij} + \sum_\nu \frac{1}{2a_\nu}\mathcal{L}_{i\nu}\mathcal{L}_{\nu j}\,. \tag{S25}$$

The term

$$-\sum_{\nu} \frac{\boldsymbol{b}_{S,\nu} \cdot \boldsymbol{b}^{E}_{S,\nu}}{2a_\nu} = -\sum_i \sum_\nu \delta\boldsymbol{\mu}_{S,\nu} \mathcal{L}_{\nu i} \boldsymbol{S}_i \,, \tag{S26}$$

describes an interaction between the strong moments and the electrically induced moments of the Co atoms mediated via the exchange with the induced Pt moments, leading to a new term in the induced effective field at the Co sites,

$$\tilde{\boldsymbol{b}}^{E}_{S,i} = \boldsymbol{b}^{E}_{S,i} + \sum_\nu \frac{1}{\mu^d_{S,i}} \mathcal{L}_{i\nu} \delta\boldsymbol{\mu}_{S,\nu} = \sum_{j(\neq i)} \frac{1}{\mu^d_{S,i}\mu^d_{S,j}} \mathcal{J}_{ij} \delta\boldsymbol{\mu}_{S,j} + \sum_\nu \frac{1}{\mu^d_{S,i}} \mathcal{L}_{i\nu} \delta\boldsymbol{\mu}_{S,\nu} \,. \tag{S27}$$

The contribution of the spin-orbit interaction that depends on the strong spin moments $\boldsymbol{S}_i$ can be written as

$$\mathcal{H}_{\rm SOC}(\{\boldsymbol{S}_i\}, \boldsymbol{E}) \simeq \sum_i \frac{\zeta_i}{2\mu_{\rm B}^2} \mu^d_{S,i} \boldsymbol{S}_i \cdot \delta\boldsymbol{\mu}_{L,i} - \sum_\nu \frac{\boldsymbol{b}_{S,\nu} \cdot \boldsymbol{b}^{E}_{L,\nu}}{2a_\nu} = -\sum_i \mu^d_{S,i}\, \tilde{\boldsymbol{b}}^{E}_{L,i} \cdot \boldsymbol{S}_i \,, \tag{S28}$$

where

$$\tilde{\boldsymbol{b}}^{E}_{L,i} = -\frac{\zeta_i}{2\mu_{\rm B}^2} \delta\boldsymbol{\mu}_{L,i} + \frac{1}{\mu^d_{S,i}} \sum_\nu \frac{1}{2a_\nu} \frac{\zeta_\nu}{2\mu_{\rm B}^2} \delta\boldsymbol{\mu}_{L,\nu} \mathcal{L}_{\nu i} \,. \tag{S29}$$

The effective spin Hamiltonian of the Co spins can then be summarized as

$$\mathcal{H}(\{\boldsymbol{S}_i\}, \boldsymbol{E}) = \sum_i \boldsymbol{S}_i \tilde{\mathcal{K}}_i \boldsymbol{S}_i - \sum_i \frac{J^{sd}}{\mu^d_{S,i}} \delta\boldsymbol{\mu}_{S,i} \cdot \boldsymbol{S}_i - \frac{1}{2} \sum_{i\neq j} \boldsymbol{S}_i \tilde{\mathcal{J}}_{ij} \boldsymbol{S}_j - \sum_i \mu^d_{S,i} \left( \tilde{\boldsymbol{b}}^{E}_{S,i} + \tilde{\boldsymbol{b}}^{E}_{L,i} \right) \cdot \boldsymbol{S}_i \,. \tag{S30}$$

In the ferromagnetic (FM) ground state of the system with magnetization along $\boldsymbol{S}_0$ and in the absence of electric fields, the induced Pt moments are given as

$$\boldsymbol{\mu}^{\rm FM}_{S,\nu} = \frac{1}{2a_\nu} \sum_i \mathcal{L}_{\nu i} \boldsymbol{S}_0 \,. \tag{S31}$$

We can naturally assume that the induced Pt moments in the FM state are parallel to $\boldsymbol{S}_0$, thus, the magnitudes of the induced moments can be expressed as

$$|\mu^{\rm FM}_{S,\nu}| \equiv |\boldsymbol{S}_0 \boldsymbol{\mu}^{\rm FM}_{S,\nu}| = \frac{1}{2a_\nu} |\sum_i \boldsymbol{S}_0 \mathcal{L}_{\nu i} \boldsymbol{S}_0| \,, \tag{S32}$$

which implies the expression for the unknown coefficients $a_\nu$,

$$\frac{1}{2a_\nu} = \frac{|\mu^{\rm FM}_\nu|}{|\sum_i \boldsymbol{S}_0 \mathcal{L}_{\nu i} \boldsymbol{S}_0|} \,. \tag{S33}$$

Using the relationship $\mathcal{J}_{i\nu} \equiv |\mu^{\rm FM}_\nu| \mathcal{L}_{i\nu}$, the renormalized spin model parameters are given as

$$\tilde{\mathcal{K}}_i = \mathcal{K}_i - \frac{1}{2} \sum_\nu \frac{\mathcal{J}_{i\nu} \mathcal{J}_{\nu i}}{|\sum_n \boldsymbol{S}_0 \mathcal{J}_{\nu n} \boldsymbol{S}_0|} \,, \tag{S34}$$

$$\tilde{\mathcal{J}}_{ij} = \mathcal{J}_{ij} + \sum_\nu \frac{\mathcal{J}_{i\nu} \mathcal{J}_{\nu j}}{|\sum_n \boldsymbol{S}_0 \mathcal{J}_{\nu n} \boldsymbol{S}_0|} \,, \tag{S35}$$

$$\tilde{\boldsymbol{b}}^{E}_{S,i} = \sum_{j(\neq i)} \frac{1}{\mu^d_{S,i}\mu^d_{S,j}} \mathcal{J}_{ij}\, \delta\boldsymbol{\mu}_{S,j} + \sum_\nu \frac{1}{\mu^d_{S,i}\, |\mu^{\rm FM}_\nu|} \mathcal{J}_{i\nu}\, \boldsymbol{\mu}^{E}_{S,\nu} \,, \tag{S36}$$

and

$$\tilde{\boldsymbol{b}}^{E}_{L,i} = -\frac{\zeta_i}{2\mu_{\rm B}^2}\, \delta\boldsymbol{\mu}_{L,i} + \frac{1}{\mu^d_{S,i}} \sum_\nu \frac{\zeta_\nu}{2\mu_{\rm B}^2} \frac{|\mu^{\rm FM}_\nu|}{|\sum_n \boldsymbol{S}_0 \mathcal{J}_{\nu n} \boldsymbol{S}_0|} \mathcal{J}_{i\nu}\, \delta\boldsymbol{\mu}_{L,\nu} \,. \tag{S37}$$

The spin Hamiltonian can then be written in the form of Eq. (10) in the main text,

$$\mathcal{H}(\{\boldsymbol{S}_i\},\boldsymbol{E}) = \sum_i \boldsymbol{S}_i \widetilde{\mathcal{K}}_i \boldsymbol{S}_i - \sum_i J^{sd} \frac{\delta\boldsymbol{\mu}_{S,i}}{\mu^d_{S,i}} \cdot \boldsymbol{S}_i - \frac{1}{2}\sum_{i\neq j} \boldsymbol{S}_i \widetilde{\mathcal{J}}_{ij} \boldsymbol{S}_j - \sum_{i\neq j} \boldsymbol{S}_i \mathcal{J}_{ij} \frac{\delta\boldsymbol{\mu}_{S,j}}{\mu^d_{S,j}}$$
$$- \sum_{i,\nu} \delta\boldsymbol{\mu}_{S,\nu} \frac{\mathcal{J}_{\nu i}}{|\mu^{\mathrm{FM}}_\nu|} \boldsymbol{S}_i + \sum_i \frac{\zeta_i}{2\mu_B^2} \mu^d_{S,i} \delta\boldsymbol{\mu}_{L,i} \cdot \boldsymbol{S}_i + \sum_{i,\nu} \frac{\zeta_\nu}{2\mu_B^2} \frac{|\mu^{\mathrm{FM}}_\nu|}{|\sum_n \boldsymbol{S}_0 \mathcal{J}_{\nu n} \boldsymbol{S}_0|} \delta\boldsymbol{\mu}_{L,\nu} \mathcal{J}_{\nu i} \boldsymbol{S}_i \,. \tag{S38}$$

The raw spin-model parameters $\mathcal{K}_i$, $\mathcal{J}_{ij}$, and $\mathcal{L}_{i\nu}$, the spin magnetic moments $\mu^d_{S,i}$ and $\mu^{\mathrm{FM}}_\nu$ are calculated from the SKKR package [3], while the Rashba-Edelstein susceptibility tensors $\boldsymbol{\chi}^{S/L}_{i/\nu}$ are evaluated using the linear-response theory [4] implemented in the WIEN2K code [5].

## II. MAGNETIZATION DEPENDENCE OF MAGNETO-ELECTRIC SUSCEPTIBILITY FROM FIRST-PRINCIPLES CALCULATIONS

The magnetization dependence of the electrically induced moments is expressed through the magneto-electric (ME) susceptibility tensors $[\boldsymbol{\chi}]^\eta$, calculated from first principles. The tensor components were calculated from first principles for certain polar and azimuthal angles $\theta$ and $\phi$, then the coefficients $[C_n]^\eta$ were determined by fitting the appropriate analytical formula to the data based on Eq. (9) of the main text. This procedure is illustrated for the spin ME susceptibility for the interface layer of cobalt in Fig. S1.

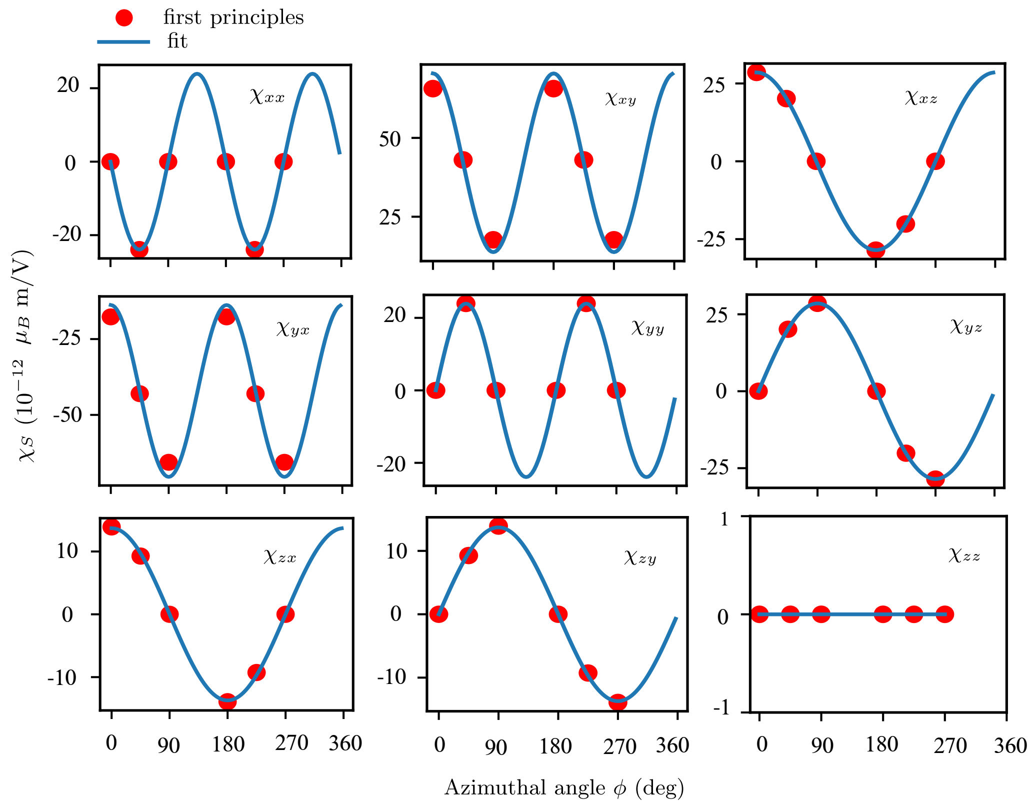


(a)

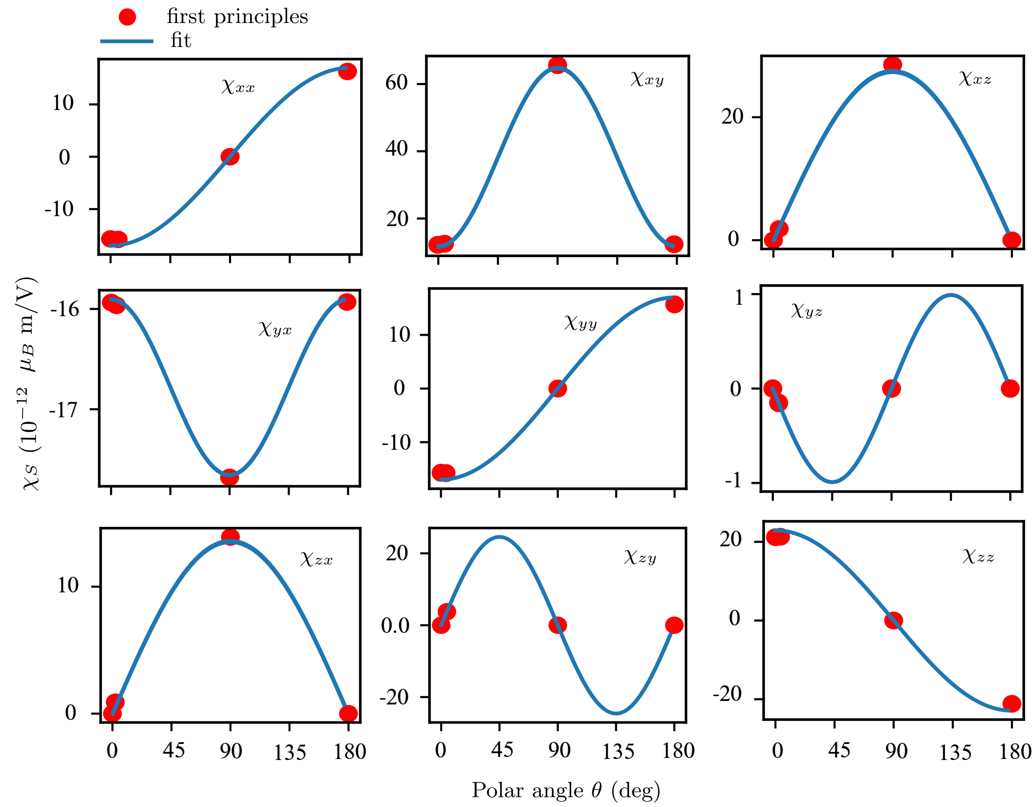


(b)

FIG. S1: *Ab initio* computed angular dependence of the spin ME susceptibility tensor components at the interface Co layer as a function of (a) magnetization azimuthal angle $\phi$ (with $\theta = \pi/2$), and (b) of the polar angle $\theta$ (for $\phi = 0$). The red symbols show the *ab initio* computed values and the blue lines are a result of the fit to the computed data using the trigonometric form of the ME tensor $\boldsymbol{\chi}^S$.

Based on Eq. (9) in the main text, the theoretical dependence of the spin ME susceptibility tensor of the Co interface layer, $[\boldsymbol{\chi}]^{\eta} = \boldsymbol{\chi}_i^S$, in Fig. S1(a) on the azimuthal angle $\phi$ (for $\theta = \pi/2$) is given as [4]:

$$[\boldsymbol{\chi}]^{\eta}(\theta=\pi/2,\phi) = \begin{bmatrix} 2[C_2]^{\eta}\sin 2\phi & ([C_3]^{\eta}+[C_4]^{\eta}) - 2[C_2]^{\eta}\cos 2\phi & [C_5]^{\eta}\cos\phi \\ -([C_3]^{\eta}+[C_4]^{\eta}) - 2[C_2]^{\eta}\cos 2\phi & -2[C_2]^{\eta}\sin 2\phi & [C_5]^{\eta}\sin\phi \\ [C_7]^{\eta}\cos\phi & [C_7]^{\eta}\sin\phi & 0 \end{bmatrix}. \tag{S39}$$

Accordingly, the theoretical dependence of the spin ME susceptibility tensor of the Co interface layer, $[\boldsymbol{\chi}]^{\eta} = \boldsymbol{\chi}_i^S$, on the polar angle $\theta$ (for $\phi = 0$), shown in Fig. S1(b), is:

$$[\boldsymbol{\chi}]^{\eta}(\theta,\phi=0) = \begin{bmatrix} [C_1]^{\eta}\cos\theta & ([C_3]^{\eta}-[C_2]^{\eta}) + ([C_2]^{\eta}-[C_4]^{\eta})\cos 2\theta & [C_5]^{\eta}\sin\theta \\ (-[C_3]^{\eta}-[C_2]^{\eta}) + ([C_2]^{\eta}+[C_4]^{\eta})\cos 2\theta & [C_1]^{\eta}\cos\theta & -[C_6]^{\eta}\sin 2\theta \\ [C_7]^{\eta}\sin\theta & -[C_8]^{\eta}\sin 2\theta & [C_9]^{\eta}\cos\theta \end{bmatrix}. \tag{S40}$$

Similarly, the magnetization dependence of the orbital ME susceptibility tensor of the Co interface layer, $[\boldsymbol{\chi}]^{\eta} = \boldsymbol{\chi}_i^L$, is shown in Fig. S2, including the fitted curves. The results are similar to the spin ME tensor but the magnitude of the respective tensor elements for the orbital ME tensor are larger comparatively.

Alternatively, the induced spin and orbital moments may also be expressed as $M$-even and $M$-odd terms as in Eqs. (14) and (15) in the main text. We consider expressions which are linear in the electric field $\boldsymbol{E}$, contain the surface normal direction $\hat{\boldsymbol{z}}$ responsible for inversion-symmetry breaking, and are up to second order in the magnetization direction $\boldsymbol{S}$.

For a magnetization direction in plane, $\boldsymbol{S}(\theta=\pi/2,\phi) = [\cos\phi,\ \sin\phi,\ 0]$, we can calculate the ME tensor elements as follows:

1. $P(A)(\boldsymbol{S}\cdot\boldsymbol{S})(\boldsymbol{E}\times\hat{\boldsymbol{z}}) = \begin{bmatrix} 0 & P(A) & 0 \\ -P(A) & 0 & 0 \\ 0 & 0 & 0 \end{bmatrix} \begin{bmatrix} E_x \\ E_y \\ E_z \end{bmatrix}$

2. $P(A')(\boldsymbol{S}\cdot\boldsymbol{E})(\boldsymbol{m}\times\hat{\boldsymbol{z}}) = P(A') \begin{bmatrix} E_x\cos\phi\sin\phi + E_y\sin^2\phi \\ -E_x\cos^2\phi - E_y\sin\phi\cos\phi \\ 0 \end{bmatrix} = \begin{bmatrix} P(A')\frac{\sin 2\phi}{2} & P(A')\frac{1-\cos 2\phi}{2} & 0 \\ -P(A')\frac{1+\cos 2\phi}{2} & -P(A')\frac{\sin 2\phi}{2} & 0 \\ 0 & 0 & 0 \end{bmatrix} \begin{bmatrix} E_x \\ E_y \\ E_z \end{bmatrix}$

3. $P(A'')\boldsymbol{m}[\boldsymbol{E}\cdot(\boldsymbol{S}\times\hat{\boldsymbol{z}})] = P(A'') \begin{bmatrix} E_x\cos\phi\sin\phi - E_y\cos^2\phi \\ E_x\sin^2\phi - E_y\sin\phi\cos\phi \\ 0 \end{bmatrix} = \begin{bmatrix} P(A'')\frac{\sin 2\phi}{2} & -P(A'')\frac{1+\cos 2\phi}{2} & 0 \\ P(A'')\frac{1-\cos 2\phi}{2} & -P(A'')\frac{\sin 2\phi}{2} & 0 \\ 0 & 0 & 0 \end{bmatrix} \begin{bmatrix} E_x \\ E_y \\ E_z \end{bmatrix}$

4. $P(A''')(\boldsymbol{E}\times\boldsymbol{S})(\boldsymbol{S}\cdot\hat{\boldsymbol{z}}) = 0$

5. $-P(B)\boldsymbol{E}(\boldsymbol{S}\cdot\hat{\boldsymbol{z}}) = 0$

6. $(P(B')+P(B))\hat{\boldsymbol{z}}(\boldsymbol{S}\cdot\boldsymbol{E}) = (P(B')+P(B)) \begin{bmatrix} 0 \\ 0 \\ E_x\cos\phi + E_y\sin\phi \end{bmatrix}$

$$= \begin{bmatrix} 0 & 0 & 0 \\ 0 & 0 & 0 \\ (P(B')+P(B))\cos\phi & (P(B')+P(B))\sin\phi & 0 \end{bmatrix} \begin{bmatrix} E_x \\ E_y \\ E_z \end{bmatrix}$$

7. $P(C)\boldsymbol{S}(\hat{\boldsymbol{z}}\cdot\boldsymbol{E}) = P(C) \begin{bmatrix} \cos\phi \\ \sin\phi \\ 0 \end{bmatrix} E_z = \begin{bmatrix} 0 & 0 & P(C)\cos\phi \\ 0 & 0 & P(C)\sin\phi \\ 0 & 0 & 0 \end{bmatrix} \begin{bmatrix} E_x \\ E_y \\ E_z \end{bmatrix}$

Combining these relations, the ME susceptibility tensor $[\boldsymbol{\chi}]^{\eta}(\theta,\phi)$ as a function of $\phi$ for $\theta = \pi/2$ is:

$$[\boldsymbol{\chi}]^{\eta}(\theta=\pi/2,\phi) = \begin{bmatrix} \frac{(P(A')+P(A''))}{2}\sin 2\phi & [\frac{(P(A')-P(A''))}{2} + P(A)] - \frac{(P(A')+P(A''))}{2}\cos 2\phi & P(C)\cos\phi \\ [\frac{(P(A'')-P(A'))}{2} - P(A)] - \frac{(P(A')+P(A''))}{2}\cos 2\phi & -\frac{(P(A')+P(A''))}{2}\sin 2\phi & P(C)\sin\phi \\ (P(B')+P(B))\cos\phi & (P(B')+P(B))\sin\phi & 0 \end{bmatrix}. \tag{S41}$$

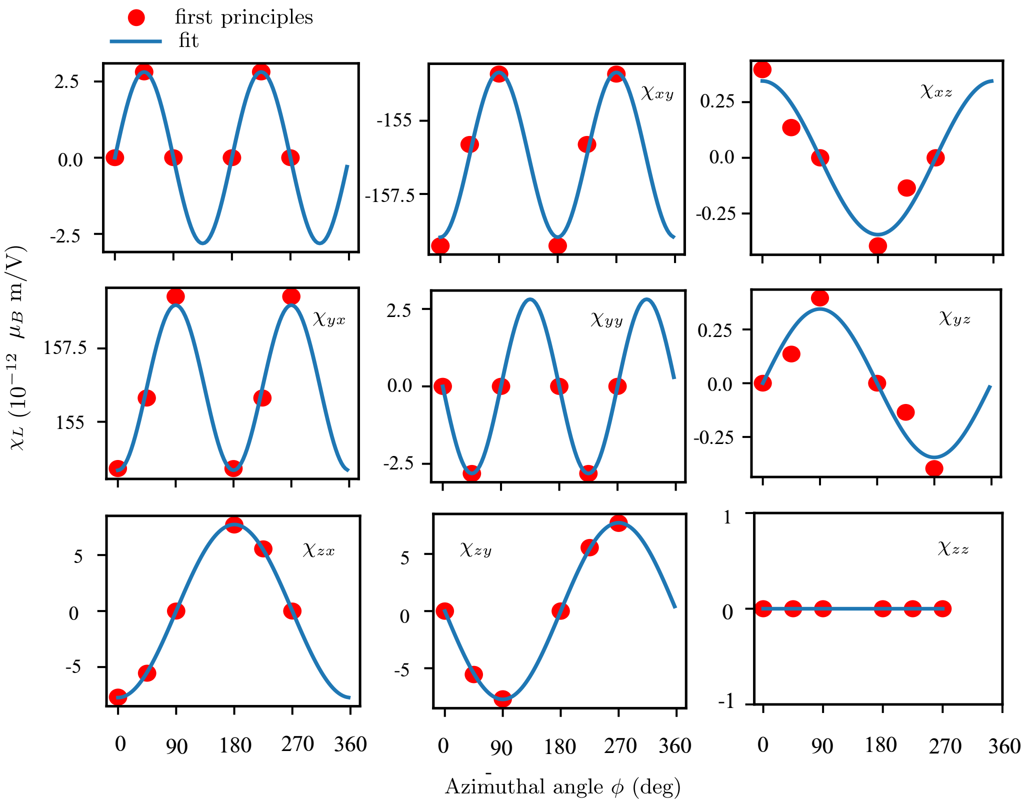


(a)

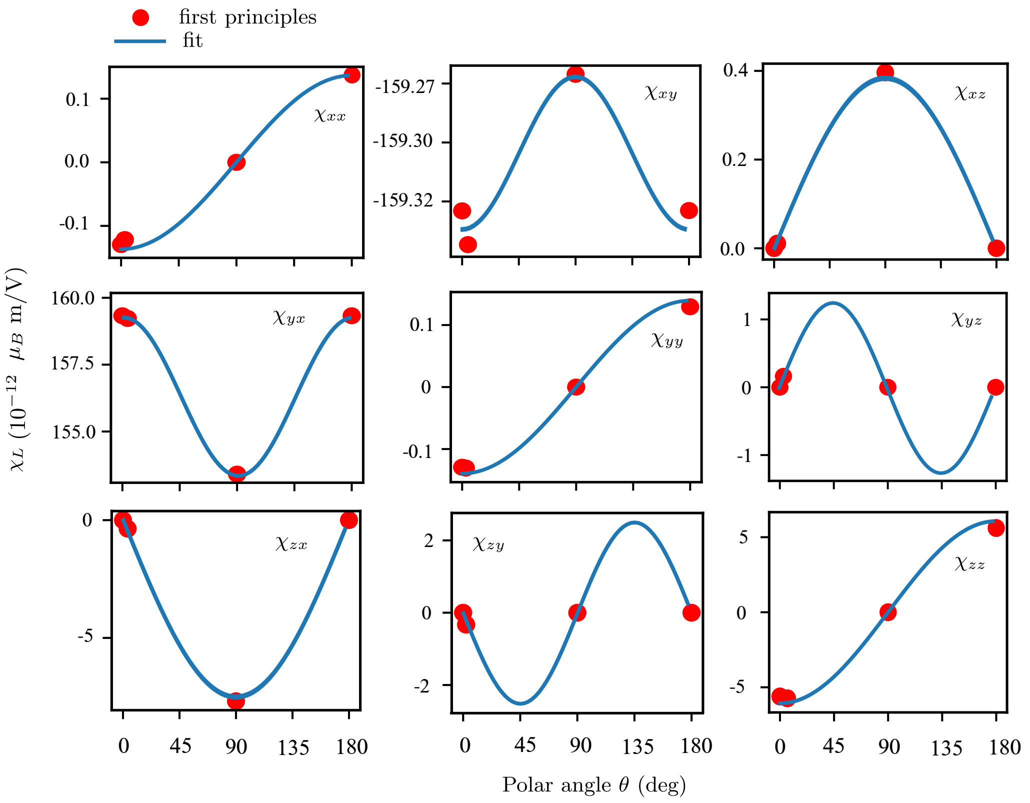


(b)

FIG. S2: Angular dependence of the orbital ME susceptibility tensor $\boldsymbol{\chi}^L(\theta,\phi)$ at the interface Co layer as a function of (a) magnetization azimuthal angle $\phi$ (for $\theta = \pi/2$), and (b) polar angle $\theta$ (for $\phi = 0$). The red symbols show the *ab initio* computed values and the blue lines are a result of the fit to the computed data using the trigonometric form of the ME tensor $\boldsymbol{\chi}^L$.

Similarly, following the above formulation, for the magnetization in the $x-z$ plane, $\boldsymbol{S}(\theta,\phi=0)=(\sin\theta,\ 0,\ \cos\theta)$ one obtains

1. $P(A)(\boldsymbol{S}\cdot\boldsymbol{S})(\boldsymbol{E}\times\hat{\boldsymbol{z}})=\begin{bmatrix}0 & P(A) & 0\\ -P(A) & 0 & 0\\ 0 & 0 & 0\end{bmatrix}\begin{bmatrix}E_x\\ E_y\\ E_z\end{bmatrix}$

2. $P(A')(\boldsymbol{S}\cdot\boldsymbol{E})(\boldsymbol{S}\times\hat{\boldsymbol{z}})=\begin{bmatrix}\frac{P(A')}{2}\sin^2\theta\sin 2\phi & P(A')\sin^2\phi\sin^2\theta & \frac{P(A')}{2}\sin\phi\sin 2\theta\\ -P(A')\cos^2\phi\sin^2\theta & -\frac{P(A')}{2}\sin^2\theta\sin 2\phi & -\frac{P(A')}{2}\sin 2\theta\cos\phi\\ 0 & 0 & 0\end{bmatrix}\begin{bmatrix}E_x\\ E_y\\ E_z\end{bmatrix}$

3. $P(A'')\boldsymbol{S}\left[\boldsymbol{E}\cdot(\boldsymbol{S}\times\hat{\boldsymbol{z}})\right]=\begin{bmatrix}\frac{P(A'')}{2}\sin^2\theta\sin 2\phi & -P(A'')\cos^2\phi\sin^2\theta & 0\\ P(A'')\sin^2\phi\sin^2\theta & -\frac{P(A'')}{2}\sin^2\theta\sin 2\phi & 0\\ \frac{P(A'')}{2}\sin\phi\sin 2\theta & -\frac{P(A'')}{2}\sin 2\theta\cos\phi & 0\end{bmatrix}\begin{bmatrix}E_x\\ E_y\\ E_z\end{bmatrix}$

4. $P(A''')(\boldsymbol{E}\times\boldsymbol{S})(\boldsymbol{S}\cdot\hat{\boldsymbol{z}})=P(A''')\begin{bmatrix}0 & \cos^2\theta & -\frac{\sin 2\theta\sin\phi}{2}\\ -\cos^2\theta & 0 & \frac{\sin 2\theta\cos\phi}{2}\\ \frac{\sin 2\theta\sin\phi}{2} & -\frac{\sin 2\theta\cos\phi}{2} & 0\end{bmatrix}\begin{bmatrix}E_x\\ E_y\\ E_z\end{bmatrix}$

5. $-P(B)\boldsymbol{E}(\boldsymbol{S}\cdot\hat{\boldsymbol{z}})=\begin{bmatrix}-P(B)\cos\theta & 0 & 0\\ 0 & -P(B)\cos\theta & 0\\ 0 & 0 & -P(B)\cos\theta\end{bmatrix}\begin{bmatrix}E_x\\ E_y\\ E_z\end{bmatrix}$

6. $(P(B')+P(B))\hat{\boldsymbol{z}}(\boldsymbol{S}\cdot\boldsymbol{E})=\begin{bmatrix}0 & 0 & 0\\ 0 & 0 & 0\\ (P(B')+P(B))\sin\theta\cos\phi & (P(B')+P(B))\sin\theta\sin\phi & (P(B')+P(B))\cos\theta\end{bmatrix}\begin{bmatrix}E_x\\ E_y\\ E_z\end{bmatrix}$

7. $P(C)\boldsymbol{S}(\hat{\boldsymbol{z}}\cdot\boldsymbol{E})=\begin{bmatrix}0 & 0 & P(C)\cos\phi\sin\theta\\ 0 & 0 & P(C)\sin\phi\sin\theta\\ 0 & 0 & P(C)\cos\theta\end{bmatrix}\begin{bmatrix}E_x\\ E_y\\ E_z\end{bmatrix}$

The ME susceptibility tensor as a function of polar angle can be written as:

$$[\boldsymbol{\chi}]^\eta(\theta,\phi=0)=\begin{bmatrix}-P(B)\cos\theta & [\frac{(P(A''')-P(A''))}{2}+P(A)]+\frac{(P(A''')+P(A''))}{2}\cos 2\theta & P(C)\sin\theta\\ -[\frac{(P(A''')+P(A'))}{2}+P(A)]+\frac{(P(A')-P(A'''))}{2}\cos 2\theta & -P(B)\cos\theta & \frac{-P(A')+P(A''')}{2}\sin 2\theta\\ (P(B')+P(B))\sin\theta & \frac{-P(A'')-P(A''')}{2}\sin 2\theta & [(P(C)+P(B'))]\cos\theta\end{bmatrix}. \tag{S42}$$

Comparing the two different formulations of the susceptibility tensors, the $[C_n]^\eta$ coefficients are related to the $P$ coefficients as follows:
$[C_1]^\eta=-P(B)$
$[C_2]^\eta=\frac{P(A')+P(A'')}{4}$
$[C_3]^\eta=\frac{P(A')-P(A'')}{4}+P(A)+\frac{P(A''')}{2}$
$[C_4]^\eta=\frac{P(A')-P(A'')-2P(A''')}{4}$
$[C_5]^\eta=P(C)$
$[C_6]^\eta=\frac{P(A')-P(A''')}{2}$
$[C_7]^\eta=P(B')+P(B)$
$[C_8]^\eta=\frac{P(A'')+P(A''')}{2}$
$[C_9]^\eta=P(C)+P(B')$.

In our case we choose the applied in-plane electric field along the $x$ direction, for which the induced spin and orbital moment vector are calculated as $\delta\boldsymbol{\mu}_S=\chi^S(\theta,\phi)\cdot\boldsymbol{E}_x=(\chi^S_{xx}E_x,\ \chi^S_{yx}E_x,\ \chi^S_{zx}E_x)$ and $\delta\boldsymbol{\mu}_L=\chi^L(\theta,\phi)\cdot\boldsymbol{E}_x=(\chi^L_{xx}E_x,\ \chi^L_{yx}E_x,\ \chi^L_{zx}E_x)$, respectively. The coefficient $P(C)$ describes a type of $M$-odd induced moment which vanishes

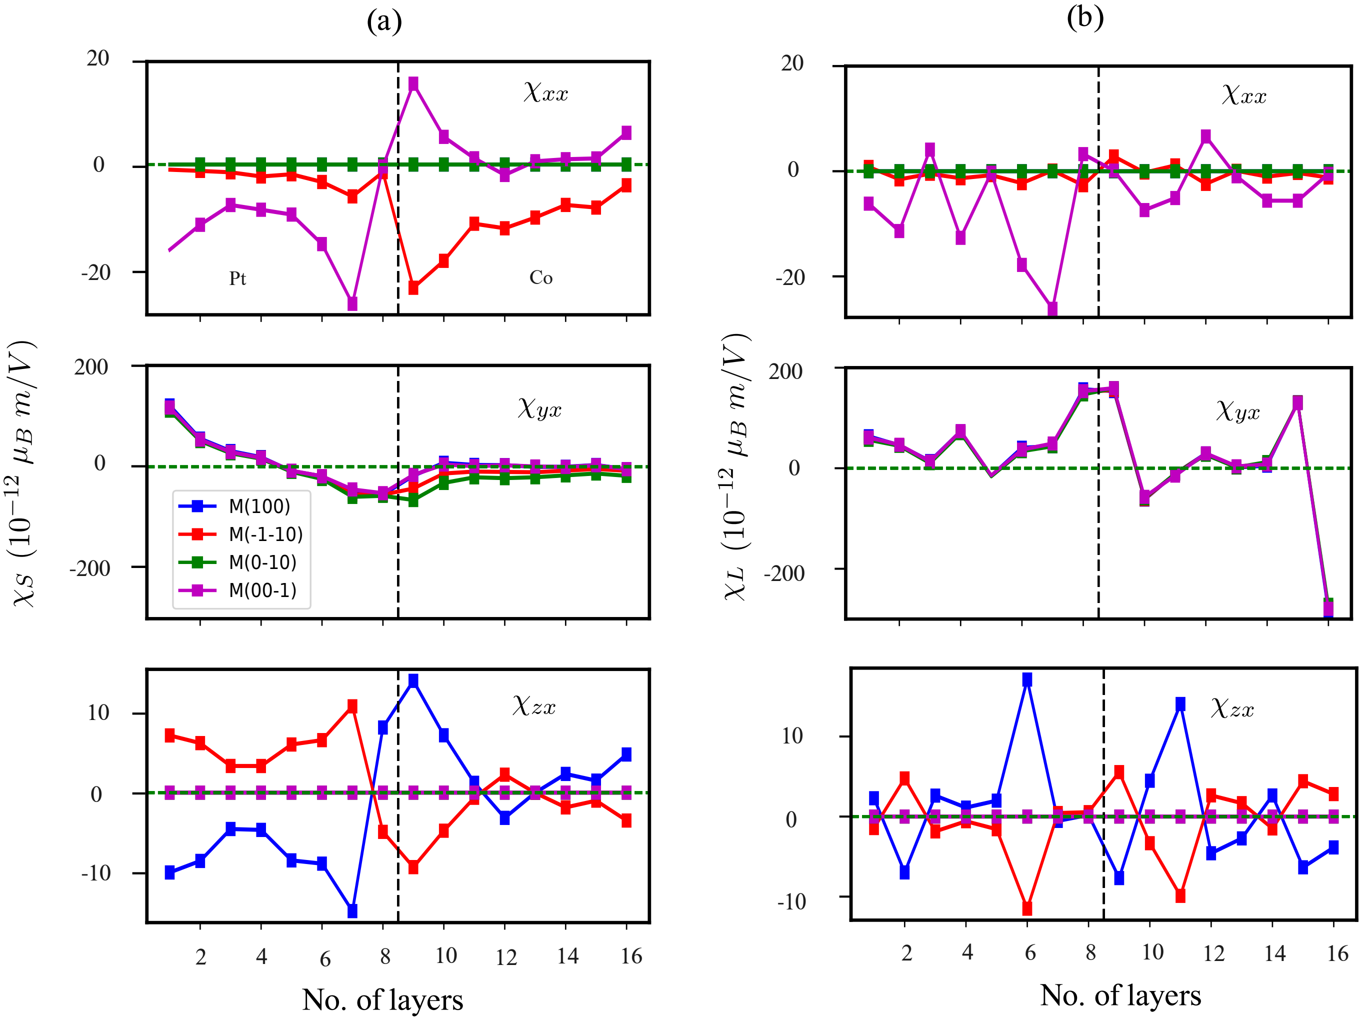


FIG. S3: First-principles layer-resolved (a) spin and (b) orbital ME susceptibility tensor components computed for an electric field $E$ in $(1,0,0)$ direction and for various magnetization directions.

for in-plane electric fields; therefore, it was not considered in the main text. In Fig. S3 the *ab initio* layer-resolved induced spin and orbital moment components for $\boldsymbol{E} = \hat{\boldsymbol{u}}_x$ are plotted for different magnetization directions.

## III. SEMI-CLASSICAL TREATMENT OF THE SPIN-ORBIT COUPLING TERM

The spin-orbit Hamiltonian terms for the system in equilibrium can be written as

$$\hat{\mathcal{H}}_{\rm SOC}(\{\hat{\boldsymbol{S}}_i\}) = \sum_i (\zeta_i/\hbar^2)\hat{\boldsymbol{L}}_i \cdot \hat{\boldsymbol{S}}_i \quad \text{and} \quad \hat{\mathcal{H}}_{\rm SOC}(\{\hat{\boldsymbol{S}}_\nu\}) = \sum_\nu (\zeta_\nu/\hbar^2)\hat{\boldsymbol{L}}_\nu \cdot \hat{\boldsymbol{S}}_\nu, \tag{S43}$$

where the first term gives the spin-orbit coupling for the spin and orbital operators pertaining to the Co atoms and the second term those for the Pt atoms. The coupling constants $\zeta_i$ and $\zeta_\nu$ (in energy units) are obtained from our *ab initio* calculations. To derive the equations of motion for the atomic spin moments under a driving field, we include the electric-field induced angular moments and make a mean-field approximation,

$$\begin{aligned}\hat{\mathcal{H}}_{\rm SOC}(\{\hat{\boldsymbol{S}}_i\},\{\delta\hat{\boldsymbol{S}}_i\},\{\delta\hat{\boldsymbol{L}}_i\}) &\approx \sum_i \zeta_i \frac{1}{2\hbar^2}\{\langle \hat{\boldsymbol{L}}_i + \delta\hat{\boldsymbol{L}}_i\rangle \cdot (\hat{\boldsymbol{S}}_i + \delta\hat{\boldsymbol{S}}_i) + (\hat{\boldsymbol{L}}_i + \delta\hat{\boldsymbol{L}}_i)\cdot\langle \hat{\boldsymbol{S}}_i + \delta\hat{\boldsymbol{S}}_i\rangle\} \\ &\approx \sum_i \zeta_i \frac{1}{2\hbar^2}\{\langle \hat{\boldsymbol{L}}_i\rangle \cdot (\hat{\boldsymbol{S}}_i + \delta\hat{\boldsymbol{S}}_i) + (\hat{\boldsymbol{L}}_i + \delta\hat{\boldsymbol{L}}_i)\cdot\langle \hat{\boldsymbol{S}}_i\rangle + \langle\delta\hat{\boldsymbol{L}}_i\rangle\cdot\hat{\boldsymbol{S}}_i + \hat{\boldsymbol{L}}_i\cdot\langle\delta\hat{\boldsymbol{S}}_i\rangle\},\end{aligned} \tag{S44}$$

where we omitted the terms quadratic in the induced angular moments; a similar derivation can be done for the Pt atoms. The Heisenberg dynamics for an atomic Co spin due to spin-orbit interaction can then be obtained from

$$\frac{d\langle\hat{\boldsymbol{S}}_i\rangle}{dt} = -\frac{i}{\hbar}\langle[\hat{\boldsymbol{S}}_i, \hat{\mathcal{H}}_{\mathrm{SOC}}(\{\hat{\boldsymbol{S}}_i\}, \{\delta\hat{\boldsymbol{S}}_i\}, \{\delta\hat{\boldsymbol{L}}_i\})]\rangle = -\frac{\zeta_i}{2\hbar^2}\langle\hat{\boldsymbol{S}}_i\rangle \times (\langle\hat{\boldsymbol{L}}_i\rangle + \langle\delta\hat{\boldsymbol{L}}_i\rangle), \tag{S45}$$

where the current-induced SOT in which we are interested arises from the $\langle\delta\hat{\boldsymbol{L}}_i\rangle$ term. Considering now only the SOT working on the Co spins, we can introduce the atomic spin and orbital magnetic moments, $\boldsymbol{\mu}_{S,i} = -2\langle\hat{\boldsymbol{S}}_i\rangle\mu_{\mathrm{B}}/\hbar$ and $\delta\boldsymbol{\mu}_{L,i} = -\langle\delta\hat{\boldsymbol{L}}_i\rangle\mu_{\mathrm{B}}/\hbar$, and use $\boldsymbol{\mu}_{S,i} = \mu^d_{S,i}\boldsymbol{S}_i$ to obtain the magnetic moment dynamics for the spin unit vector due to the SOT, as

$$\left.\frac{d\boldsymbol{S}_i}{dt}\right|_{\mathrm{SOT}} = -\frac{\gamma}{\mu^d_{S,i}}\left[\boldsymbol{S}_i \times \left(-\frac{\zeta_i\mu^d_{S,i}\delta\boldsymbol{\mu}_{L,i}}{2\mu_{\mathrm{B}}^2}\right)\right] = -\frac{\gamma}{\mu^d_{S,i}}\left[\boldsymbol{S}_i \times \left(-\frac{\partial\mathcal{H}^{\mathrm{ind}}_{\mathrm{SOC}}}{\partial\boldsymbol{S}_i}\right)\right]. \tag{S46}$$

From this we recognize that the expression for the electric-field induced spin-orbit coupling term in the classical spin Hamiltonian is

$$\mathcal{H}^{\mathrm{ind}}_{\mathrm{SOC}}(\{\boldsymbol{S}_i\}, \{\delta\boldsymbol{\mu}_{L,i}\}) = \sum_i \frac{\zeta_i}{2\mu_{\mathrm{B}}^2}\mu^d_{S,i}\boldsymbol{S}_i \cdot \delta\boldsymbol{\mu}_{L,i}, \tag{S47}$$

which is the expression given for the Co atoms in Eq. (12) of the main text. An equivalent expression can be derived for the Pt atoms.

From first-principles calculations we obtained $\zeta_{\mathrm{Co}} = 90.75$ meV and $\zeta_{\mathrm{Pt}} = 601.4$ meV. Note that, since we consider here only LLG spin dynamics, no dynamics of the orbital magnetic moment $\boldsymbol{\mu}_{L,i}$ is included.

## IV. LAYER-RESOLVED MAGNETOCRYSTALLINE ANISOTROPY

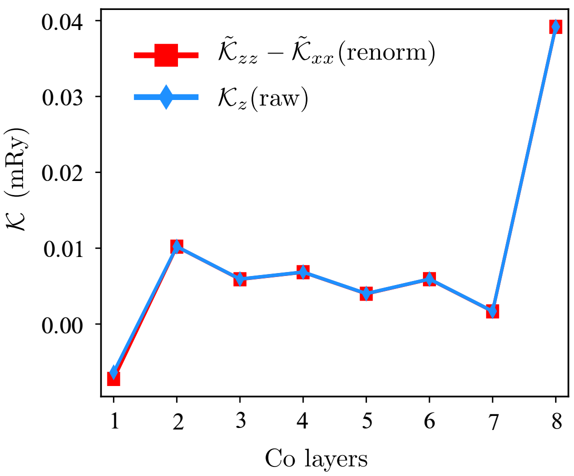


FIG. S4: The anisotropy constant obtained after renormalization (red symbols) is compared with the *ab initio* computed raw value (blue symbols)

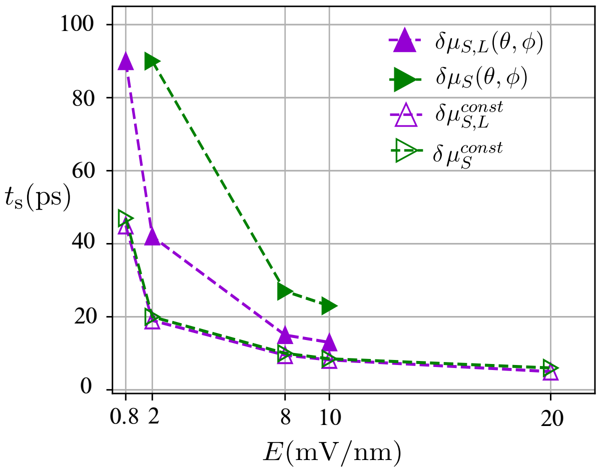


FIG. S5: Computed switching time $t_{\mathrm{s}}$ analyzed for the following four cases: magnetization dependent ($\delta\mu_{S,L}(\theta,\phi)$) and independent ($\delta\mu^{\mathrm{const}}_{S,L}$) induced spin moments, either in the absence (green) or presence (purple) of induced orbital moments as a function of the electric-field magnitude.

The *ab initio* calculated magnetocrystalline anisotropy energy in the 8 cobalt layers is shown in Fig. S4, where the renormalized anisotropy constant ($\tilde{\mathcal{K}}_{zz} - \tilde{\mathcal{K}}_{xx}$) in Eq. (S24) is compared with the raw anisotropy parameter in cobalt layers ($\mathcal{K}_{zz} - \mathcal{K}_{xx}$). The figure shows that the renormalization only has a visible, but still quite small, effect at the interface with Pt. It can also be seen that the largest anisotropy contribution is coming from vacuum surface (8th layer). The positive values of the anisotropy constants apart from the interface layer indicate an easy-plane anisotropy in the system.

## V. SWITCHING TIMES

The magnetic switching time is analyzed considering magnetization-independent moments ($\delta\mu_{S,L}^{\mathrm{const}}$) as well as magnetization-dependent moments ($\delta\mu_{S,L}(\theta,\phi)$), in each case with the presence or absence of induced orbital moments in addition to induced spin moments, while varying the electric field magnitude in the range $0.8-20\,\mathrm{mV/nm}$. The results of the simulations are shown in Fig. S5. Here, the switching time is defined as the time taken by the magnetization to reach the $\boldsymbol{E}\times\hat{\boldsymbol{z}}$ direction (i.e., $-\hat{\boldsymbol{y}}$ here) at first on application of the electric field. It can be seen that the switching time for magnetization independent moments is similar in the presence and absence of induced orbital moments, whereas in the case of including magnetization-dependent moments a clear difference in switching time can be observed between the presence and absence of induced orbital moments. Note that there are no data points for cases where switching does not occur for a given electric field value. As observed before, the presence of the induced orbital moments leads to a faster switching.

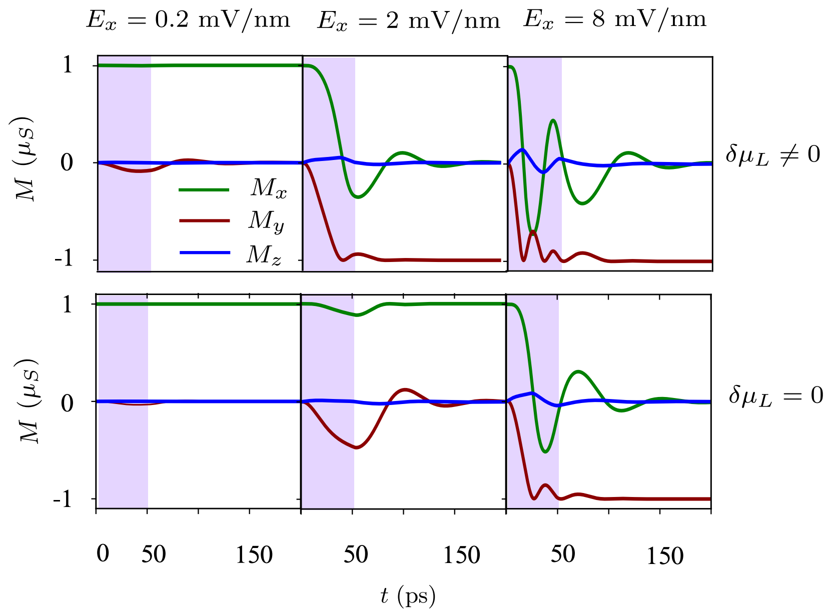


FIG. S6: Calculated magnetization switching at $T=0\,\mathrm{K}$ for the easy-plane anisotropic Co layers in the presence (top) and absence (bottom) of the induced orbital moments when applying a 50-ps-long rectangular electric field pulse with magnitude $E_x = 0.2,\ 2$ and $8$ mV/nm.

## VI. MAGNETIZATION DYNAMICS AT $T=0\,\mathrm{K}$

In Fig. S6 we show spin-dynamics simulations performed at $T=0\,\mathrm{K}$ in the system when applying a 50-ps-long rectangular electric field pulse in the $\hat{x}$ direction, with the initial magnetization condition $\boldsymbol{M}\,||\,\boldsymbol{E}$. It can be observed that the presence of induced orbital moments leads to magnetization switching at smaller electric field magnitude ($E=2$ mV/nm) where the influence of the induced spin moments alone is too weak to induce switching. Furthermore, at higher electric field ($E=8$ mV/nm), the strong effect of the induced orbital moments can be seen in the faster switching time (12 ps) as compared to the simulation when turning the induced orbital moments off (25 ps).

## VII. IMPORTANCE OF INDUCED PT MOMENTS AND ROLE OF SURFACE IN THE SWITCHING DYNAMICS

To understand the importance of interaction terms with induced spin and orbital Pt moments at the interface, we have simulated the system while turning off these renormalization interaction terms. We observe from Fig. S7 (left) that the magnetization moves in opposite direction and switching does not occur on larger time scales. This shows that renormalization terms are important to see switching at lower fields. Since we have opposite current-induced orbital moments at the Co/vacuum surface, we therefore also simulate the system while turning off the induced surface

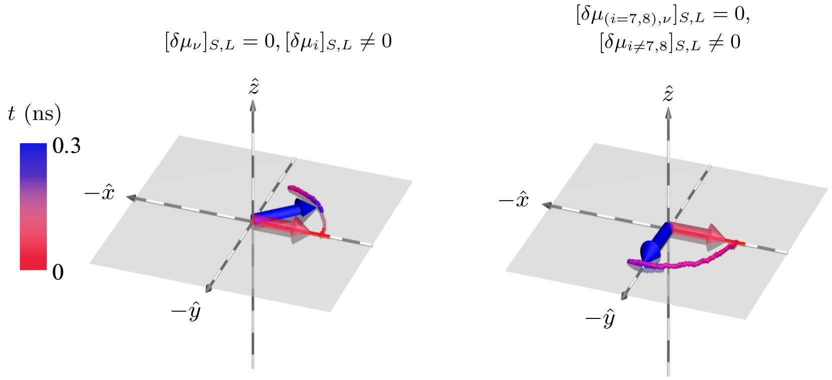


FIG. S7: Magnetization dynamics at $E_x = 0.8$ mV/nm calculated for absence of electrically induced interface Pt moments (left) and absence of both interface Pt moments and induced moments at the Co/vacuum surface (right) as written in the headings.

moments in absence of Pt-renormalization terms. We observe from Fig. S7(right) that now switching occurres from interface Co moments but at a slower rate. To clearly understand the torque acting in these conditions we have analyzed the field-like torque acting on Co films and averaged it over the Co atoms in the Co film; the results are shown in Fig. S8 and compared for different assumptions on the induced moments. From Sec. III B of the main text, it is known that only field-like torque drives the switching dynamics, therefore we compare only field-like torques. Focusing on the total SOT ($T^{\text{SOT}}_{\text{total}}$) in Fig. S8, the largest SOT occurs on omitting the induced moments at the Co/vacuum surface with presence of renormalization interaction with electrically induced moments at interface-Pt layer, this in turn leads to faster switching at lower electric field magnitude. The switching time is compared in Fig. S9. From this figure, we observe that switching also occurs at even lower electric field magnitude ($E_x = 0.4$ and 0.6 mV/nm) in absence of the Co/vacuum surface moments and has lower switching time at a given electric field when compared with cases where switching occurs in the presence of Co/vacuum surface moments.

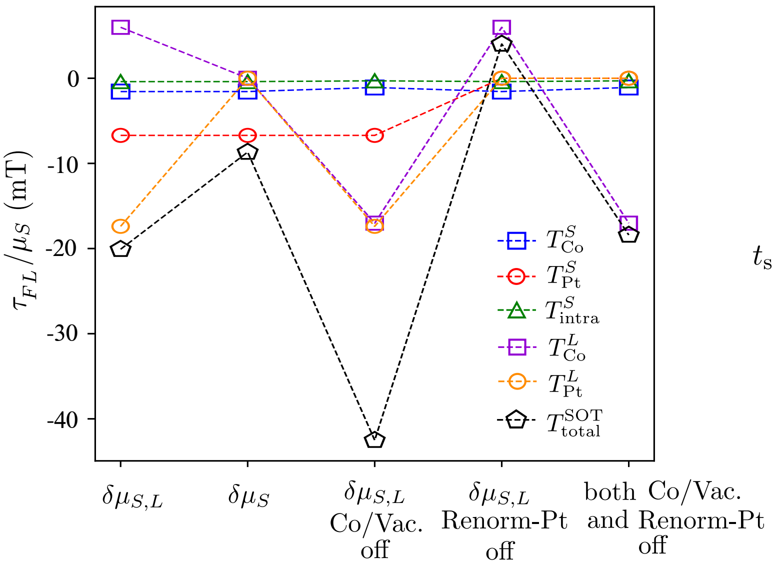


FIG. S8: Average initial field-like torque computed for different assumptions on the induced moments as depicted on the x-axis at $E_x = 0.8$ mV/nm.

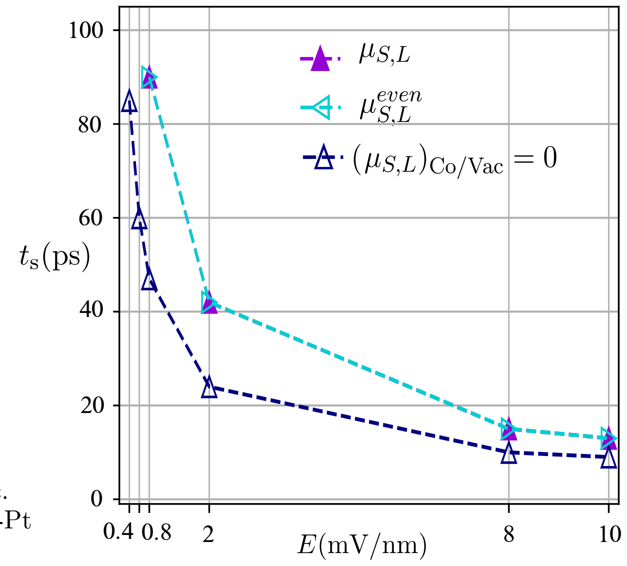


FIG. S9: Switching time versus electric field magnitude computed in the presence of the total torque, the $M$-even torque, and total torque in the absence of electrically induced moments at the Co/vacuum surface.

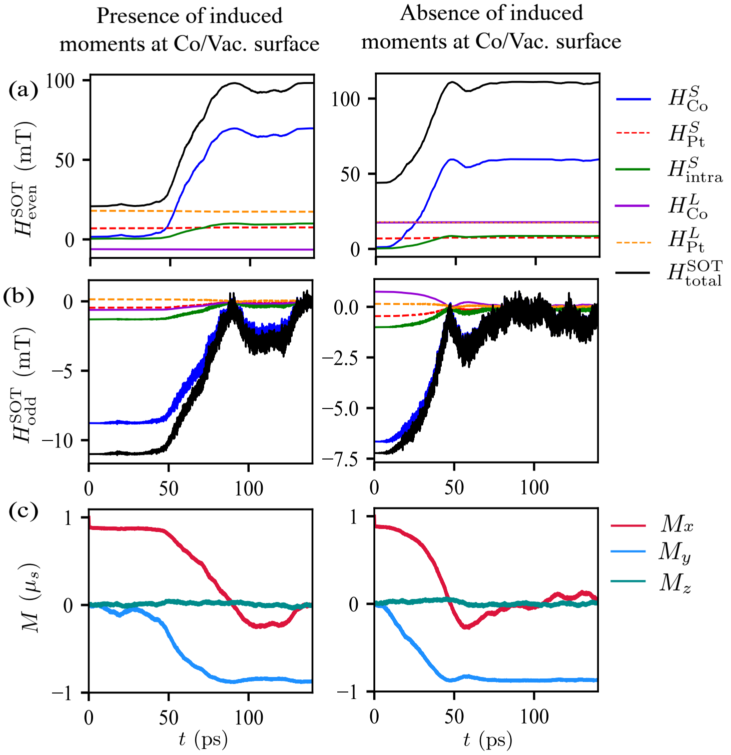


FIG. S10: The dynamics of the (a) $M$-even ($\boldsymbol{E} \times \hat{\boldsymbol{z}}$) and (b) $M$-odd ($\boldsymbol{S} \times \boldsymbol{E} \times \hat{\boldsymbol{z}}$) SOT field are analyzed in the presence or absence of induced moments at the Co/vacuum surface. Panel (c) shows the corresponding magnetization dynamics.

## VIII. SOT-FIELD DYNAMICS WITH MAGNETIZATION DEPENDENCE

The dynamical SOT-field is analyzed for the SOT contributions given in Eq. (13) in the main text. The $M$-even ($\boldsymbol{E} \times \hat{\boldsymbol{z}}$) SOT field ($H^{\rm SOT}_{\rm even}$) which applies a field-like torque and the $M$-odd ($\boldsymbol{S} \times \boldsymbol{E} \times \hat{\boldsymbol{z}}$) SOT field ($H^{\rm SOT}_{\rm odd}$) which applies an anti-damping torque are shown in Fig. S10 for two cases, when current-induced moments are present at the Co/vacuum surface (left) and when they are absent (right). Focusing on the $M$-even SOT field, it can be seen that initially for $\boldsymbol{S} \,||\, \boldsymbol{E}$, the SOT field from induced orbital moments ($H^L_{\rm Co}, H^L_{\rm Pt}$) is stronger than the SOT field from induced spin moments ($H^S_{\rm Co}$). But as $\boldsymbol{S}$ switches parallel to $\boldsymbol{E} \times \hat{\boldsymbol{z}}$ direction, the SOT field from spin induced moments gets stronger than induced orbital moments, whereas there is negligible change in strength of SOT-field from orbital moments. Since the SOT-field from $M$-even induced moments contains a mix of magnetization dependent (terms with $P(A'')$, $P(A''')$ and $P(A')$) and independent ($P(A)$) terms, the variation in strength of the induced spin moments with change in in-plane magnetization directions signifies the stronger magnetization direction dependence of induced spin moments, where weak induced spin moment for $\boldsymbol{S} \,||\, \boldsymbol{E}$ (or $\boldsymbol{S}$ perpendicular to $\boldsymbol{E} \times \hat{\boldsymbol{z}}$) and larger strength at $\boldsymbol{S} \,||\, (\boldsymbol{E} \times \hat{\boldsymbol{z}})$ is attributed to spin scattering and spin filtering at interface, whereas almost constant magnitude of SOT field from induced orbital moments for $\boldsymbol{S} \,||\, \boldsymbol{E}$ and $\boldsymbol{S} \,||\, \boldsymbol{E} \times \hat{\boldsymbol{z}}$ depicts the advantage of induced orbital moments that there is no such orbital moment loss due to the interface effect. Therefore, we conclude that orbital moments are either strongly $M$-independent and have very small contributions from $M$-dependence leading to no loss in orbital moments at interface or have closely similar contributions corresponding to different in-plane magnetization directions in case of $M$-even moments. Now based on this observation, the scaling parameter $t_m$ we used to separate $M$-dependent and $M$-independent induced moments given in analytical formulation Eq. (14) in the manuscript, can be verified, and for induced spin moments our assumed value $t_m = -1$ matches for induced spin moments, as total contribution from induced spin moments gets higher at $\boldsymbol{S} \,||\, (\boldsymbol{E} \times \hat{\boldsymbol{z}})$ and for orbital moments the $t_m$ is either equal to $-1$ or between $-1$ to 0.

[1] O. N. Mryasov, Magnetic interactions and phase transformations in FeM, M=(Pt, Rh) ordered alloys, Phase Transitions **78**, 197 (2005).
[2] M. Ležaić, P. Mavropoulos, G. Bihlmayer, and S. Blügel, Exchange interactions and local-moment fluctuation corrections in ferromagnets at finite temperatures based on noncollinear density-functional calculations, Phys. Rev. B **88**, 134403 (2013).
[3] J. Zabloudil, R. Hammerling, L. Szunyogh, and P. Weinberger, *Electron Scattering in Solid Matter: A Theoretical and Computational Treatise*, Springer Series in Solid-State Sciences No. 147 (Springer-Verlag, Berlin Heidelberg, 2005).
[4] L. Salemi, M. Berritta, and P. M. Oppeneer, Quantitative comparison of electrically induced spin and orbital polarizations in heavy-metal/3*d*-metal bilayers, Phys. Rev. Mater. **5**, 074407 (2021).
[5] P. Blaha, K. Schwarz, G. K. H. Madsen, D. Kvasnicka, J. Luitz, R. Laskowsk, F. Tran, and L. Marks, *WIEN2k: An Augmented Plane Wave Plus Local Orbitals Program for Calculating Crystal Properties* (Techn. Universitat, 2019) user's Guide, WIEN2k 19.1. Available online: `http://susi.theochem.tuwien.ac.at/reg_user/textbooks/usersguide.pdf`.
